# Supplementary material for: Real-time Model Predictive Control and System Identification Using Differentiable Physics Simulation
Source: arXiv:2202.09834 source file (2022-11-23)
Supplement: Supplementary file 1 [file appendix.tex]

\section{Appendix}
\subsection{Details of MPC-iLQR Algorithm}
\label{subsec:MPC}
We show the algorithm of our implementation of MPC-iLQR in Algorithm \ref{alg:MPC-iLQR}. Please see \cite{iLQR} for detailed derivation of iLQR. $\bm{u}_t$ is control force at time $t$, and $\bm{K}_t, \bm{k}_t$ are feedback and feedforward gain in iLQR algorithm. We use warm start for iLQR trajectory optimizer. At the beginning of the algorithm, the buffer for state, action, feedback and feedforward gain are initialized using last iLQR buffer with obsolete terms discarded. When deploying the algorihm, we use $\Tilde{\bm{u}}_t = \bm{u}_t + \bm{K}_t\bm{x}_t+\bm{k}_t$ to compute control forces $\Tilde{\bm{u}}_t$ based on actual observed state $\bm{x}_t$.

\begin{algorithm}[b!]
\caption{MPC-iLQR}
\KwIn{$\bm{x}_{\hat{t}}$, $\bm{\bar{\mu}}$, $f$, $H$, $\epsilon$, $N_\text{maxiter}$} 
$i = 0$\\
$c_\text{old}, c_\text{new}=\mathrm{Inf}$\\
\Comment{Initialize from last optimization} \\
$H_\text{last\ remain} \longleftarrow t_\mathrm{last\ end} - \hat{t} $\\
$\bm{u}_{\hat{t}:\hat{t}+\mathcal{H}_\mathrm{last\ remain}} \longleftarrow \bm{u}_{t_\mathrm{last\ end} - t_\mathrm{last\ remain}}$\\
$\bm{k}_{\hat{t}:\hat{t}+\mathcal{H}_\mathrm{last\ remain}} \longleftarrow \bm{k}_{t_\mathrm{last\ end} - t_\mathrm{last\ remain}}$\\
$\bm{K}_{\hat{t}:\hat{t}+\mathcal{H}_\text{last\ remain}} \longleftarrow \bm{K}_{t_\text{last\ end} - t_\text{last\ remain}}$\\
$\bm{x}_{\hat{t}:\hat{t}+\mathcal{H}_\text{last\ remain}} \longleftarrow \bm{x}_{t_\text{last\ end} - t_\text{last\ remain}}$\\
\Comment{Optimize trajectory using iLQR:} \\
\While{$i < N_\mathrm{maxiter}$}
{
    $c_\text{new}, \bm{x}_{\hat{t}:\hat{t}+H}, \bm{A}_{\hat{t}:\hat{t}+H}, \bm{B}_{\hat{t}:\hat{t}+H} \longleftarrow \mathrm{iLQRForward}(\bar{\bm{\mu}},f)$\\
    $\bm{u}_{\hat{t}:\hat{t}+H-1}, \bm{k}_{\hat{t}:\hat{t}+H-1}, \bm{K}_{\hat{t}:\hat{t}+H-1} \longleftarrow \mathrm{iLQRBackward}(f)$\\
    \If{$|c_\mathrm{new} - c_\mathrm{new}| \le \epsilon$}
    {
    \textbf{Terminate}\\
    }
    $c_\text{old} \longleftarrow c_\text{new}$\\
    $i \longleftarrow i+1$
}
\label{alg:MPC-iLQR}
\end{algorithm}

\subsection{Coriolis terms}
\label{subsec:coriolis}
Corilios and centrifugal forces can be added to the computation of the confidence score in mass and moment of inertia estimation. Our method achieves good results without including this term, but it might improve the results for more dynamic and complex examples.
\[
\bm{c}(\bm{q},\bm{\dot{q}};\bm{\mu}) = m_k(\bm{J}_{{k}}^T\bm{\dot{J}}_{{k}} + \bm{J}_{\omega k}^T\Tilde{\bm{I}}\bm{J}_{{k}}+\bm{J}_{\omega k}^T[\bm{\omega}]\bm{\Tilde{I}}\bm{J}_{\omega k})\bm{\dot{q}}\\
\]
For mass, we can add $(\bm{J}_{{k}}^T\bm{\dot{J}}_{{k}} + \bm{J}_{\omega k}^T\bm{\Tilde{I}}\bm{J}_{{k}}+\bm{J}_{\omega k}^T[\bm{\omega}]\bm{\Tilde{I}}\bm{J}_{\omega k})\bm{\dot{q}}$ as additional term after each $\bm{B}(:,k)$. For moment of inertia, we can add $\bm{J}^T_{\omega k}[\bm{\omega}]\text{Diag}(\bm{J}_{\omega k} \bm{\dot{q}})$ after each $\bm{C}_k$, $\bm{\omega}_k = \bm{J}_{\omega k}\bm{\dot{q}}$.
